# Supplementary material for: A two-dimensional array of single-hole quantum dots
Source: arXiv:2008.11666 ancillary file (2020-08-26)
Supplement: Supplementary file 1 [file SupplementaryInformation.pdf]

# A two-dimensional array of single-hole quantum dots: Supplementary Information

F. van Riggelen,<sup>1,\*</sup> N. W. Hendrickx,<sup>1</sup> W. I. L. Lawrie,<sup>1</sup> M. Russ,<sup>1</sup> A. Sammak,<sup>2</sup> G. Scappucci,<sup>1</sup> and M. Veldhorst<sup>1,†</sup>

<sup>1</sup>*QuTech and Kavli Institute of Nanoscience, Delft University of Technology, Lorentzweg 1, 2628 CJ Delft, The Netherlands*

<sup>2</sup>*QuTech and Netherlands Organization for Applied Scientific Research (TNO), Stieltjesweg 1 2628 CK Delft, The Netherlands*

---

\* f.vanriggelen@tudelft.nl

† m.veldhorst@tudelft.nl

## I. CHARGE STABILITY DIAGRAM $Q_2$ - $Q_4$

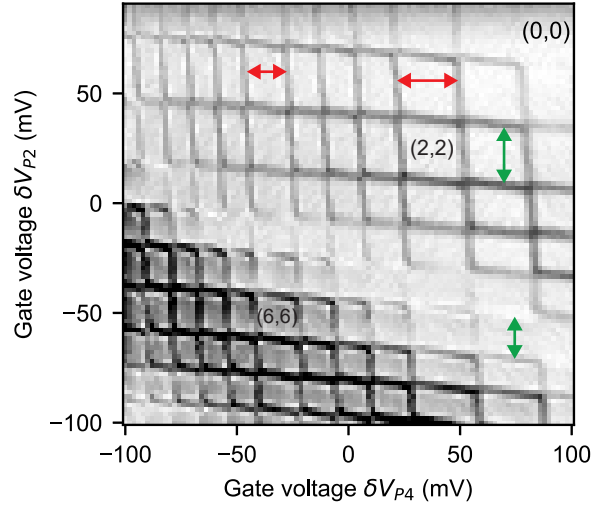

Figure 1. **Charge filling**  $Q_2 - Q_4$  Shown is a charge stability diagram of the double quantum dot  $Q_2 - Q_4$  with negligible tunnel coupling. Here the results are shown as measured with sensor  $S_2$ , the sensor closest to this quantum dot pair. The numbers added to the diagram  $(N_{Q_2}, N_{Q_4})$  indicate the hole occupancy in quantum dots  $Q_2$  and  $Q_4$  respectively. The colored arrows correspond to the hole filling for which one would expect a peak in the addition energy due to the shell filling of a quantum dot with a circular potential and spin degeneracy.

## II. VIRTUAL GATES

The data shown in Figure 3d-f of the main text was taken in a virtual gate space of detuning and energy ( $\epsilon_{34}$  and  $U_{34}$ ). The matrix defining the voltages on gates  $\epsilon_{34}$  and  $U_{34}$  as a linear combination of the voltages on gates  $P_3$  and  $P_4$  is the following:

$$\begin{pmatrix} V_{P3} \\ V_{P4} \end{pmatrix} = \begin{pmatrix} 0.5 & 0.5 \\ -0.5 & 0.5 \end{pmatrix} \begin{pmatrix} V_{\epsilon_{34}} \\ V_{U_{34}} \end{pmatrix}$$

For the data shown in Figure 4 of the main text, a virtual gate sets was defined such that for all four quantum dots the filling of  $N=1$  coincides and that the slope of the addition lines of all four dots can be distinguished from each other. The voltages on the two virtual gates  $e_{1234}$  and  $U_{1234}$  were constructed as a linear combination of the voltages on all the four plunger gates  $P_1 - P_4$ . The matrix defining the virtual gate space is the following:

$$\begin{pmatrix} V_{P1} \\ V_{P2} \\ V_{P3} \\ V_{P4} \end{pmatrix} = \begin{pmatrix} 0.65 & 1.92 \\ -0.38 & 0.38 \\ 0.66 & 0.77 \\ -0.14 & 0.42 \end{pmatrix} \begin{pmatrix} V_{e_{1234}} \\ V_{U_{1234}} \end{pmatrix}$$

During both of these measurements, the effect on the plunger gates of the sensors were also compensated.

## III. LEVER ARM

The lever arm, used to convert the applied gate voltage to the detuning energy (meV) in Figure 3e and 3f of the main text, is  $\alpha = 0.19$  eV/V. This value was obtained by performing a photon assisted tunneling (PAT) measurement [1] at the (1,1)-(0,2) anticrossing in virtual gate space of detuning and energy ( $\epsilon_{34}$ ,  $U_{34}$ ). For a PAT measurement a microwave field is used to induce the re-population of states. Resonance peaks are observed when the frequency of

the microwave source is equal to the energy difference between two states, i.e. the resonance frequency is given by  $hf = \sqrt{\epsilon^2 + 4t^2}$ , where  $h$  is Planck's constant,  $f$  is the frequency of the microwave source,  $t$  is the interdot tunneling and  $\epsilon$  is the detuning which is given by  $\alpha\delta\epsilon_{34}$ . This measurement is taken in the regime where the tunnel coupling was turned off, making the extracting of the lever arm  $\alpha$  straight forward.

To calculate the addition energies as plotted in Figure 1b from the main text, the same lever arm  $\alpha = 0.19$  eV/V was used. Since the virtual gate matrix defining  $\epsilon_{34}$  and  $U_{34}$  is symmetric for the gates  $P_3$  and  $P_4$  (see previous section) and the capacitance of the four plunger gates to the quantum dots underneath is similar (estimated from the slope of the addition lines from the charge stability diagrams shown in Figure 2a in the main text and Figure 1 in the Supplementary Information), we conclude this as a reasonable assumption.

#### IV. TUNNEL COUPLING

For fitting the extracted values for the tunnel coupling we use a model based on tunneling through a rectangular barrier. In the limit of weak tunneling the tunnel probability can be approximated by the WKB approximation, which reads for a rectangular barrier (see Supplementary Materials in Ref. [2]):

$$|t|^2 = 16c \frac{|V_B - V_0|}{(V_B - V_1)^2} \exp \left( -2b \sqrt{\frac{2m\alpha}{\hbar^2} |V_B - V_0|} \right). \quad (1)$$

Here,  $V_0$  is the voltage when the barrier height is equal to the energy of the hole,  $V_1$  is the voltage when the barrier height is zero,  $\alpha$  is the lever arm which translates the barrier voltage into energy units,  $b$  is the width of the barrier,  $m$  is the effective mass of the hole, and  $c$  is an overall scaling factor. By fitting the experimentally determined values we extract  $V_0 = -17.6$  mV,  $V_1 = -25.2$  mV, and  $b\sqrt{2m\alpha/\hbar^2} = 2.41 \frac{1}{\sqrt{\text{mV}}}$ , and  $c = 2.82 \times 10^9 \frac{\text{GHz}^2}{\text{mV}}$ .

- 
- [1] Van Diepen, C.J.; Eendebak, P.T.; Buijtenorp, B.T.; Mukhopadhyay, U.; Fujita, T.; Reichl, C.; Wegscheider, W.; Vandersypen, L.M.K. Automated tuning of inter-dot tunnel coupling in double quantum dots. *Applied Physics Letters* **2018**, *113*, 033101.
  - [2] Zajac, D.M.; Sigillito, A.J.; Russ, M.; Borjans, F.; Taylor, J.M.; Burkard, G.; Petta, J.R. Resonantly driven CNOT gate for electron spins. *Science* **2018**, *356*, 439–442.
-
